# Supplementary material for: Spectra of a class of non-self-adjoint matrices
Source: arXiv:1311.6741 ancillary file (2013-11-26)
Supplement: Supplementary file 1 [file makemovie.pdf]

```

(* This script is ancillary to the paper
by E.B.Davies and M.Levitin
"Spectra of a class of non-self-adjoint matrices" *)

In[55]:= (* this function computes the eigenvalues of the operator pencil
 $H_{m+n}$ ,  $c - \lambda D_{m+n}$ ; it returns the list of pairs  $\{\text{Re}[\lambda], \text{Im}[\lambda]\}$  *)
AmatrixEigs[m_, n_, c_] := Module[{H, Dd, i, j, ee},
  H = DiagonalMatrix[Table[c, {i, m+n}]];
  If[m+n > 1, H = H + DiagonalMatrix[Table[1, {i, m+n-1}], 1, m+n] +
    DiagonalMatrix[Table[1, {i, m+n-1}], -1, m+n]];
  Dd = DiagonalMatrix[Table[If[i ≤ m, 1, -1], {i, m+n}]];
  ee = Eigenvalues[Dd.H];
  Table[{Re[ee[[i]]], Im[ee[[i]]]}, {i, m+n}]
]

(* this function rescales the imaginary parts of
an eigenvalue list ee by N=dim(ee) *)
RescaleEigs[ee_] := Module[{i, M},
  M = N[Length[ee]];
  Table[{ee[[i, 1]], ee[[i, 2]] M}, {i, M}]
]

(* see Section 4 of the paper *)
 $\Lambda_0[u] := \text{Sqrt}[4 - u^2] \text{Log}[\text{Tan}[\text{Pi} / 4 + 1 / 2 \text{ArcCos}[u / 2]]];$ 

(* see Section 5 of the paper *)
X[c_, u_, v_] := Tanh[v / (2 Sqrt[4 - (u - c)^2])] Tanh[v / (2 Sqrt[4 - (u + c)^2])];
 $\Lambda[c_, u_] := v /. \text{FindRoot}[$ 
  X[c, u, v] == Abs[Tan[ArcCos[(u - c) / 2] / 2] Tan[ArcCos[(u + c) / 2] / 2]], {v, 2 - u}];

In[60]:= (* this function separates the list of scaled eigenvalues
into the list of the real ones and the list of the non-real ones *)
eigsRI[m_, c_] := Module[{ee},
  ee = RescaleEigs[AmatrixEigs[m, m, c]];
  {Select[ee, #[[2]] == 0 &], Select[ee, #[[2]] ≠ 0 &]}
]

```

```

In[75]:= (* this function creates one frame of the movie with
          m= mm, c=cc;
          parameters cmax and ymax determine the axes limits to help scaling;
          fsize gives the horizontal frame size in inches;
          plotest is the logical variable which determines whether or not to plot
          the asymptotic estimates *)
OneFrame[mm_, cc_, cmax_, ymax_, fsize_, plotest_] :=
Module[
  {ri, st, pllist, stlist, lplot, eplot},
  ri = eigsRI[mm, N[cc]];
  st = {Blue, Red};
  If[ri[[1]] == {},
    (pllist = {ri[[2]]}; stlist = {st[[2]]});,
    If[ri[[2]] == {},
      (pllist = {ri[[1]]}; stlist = {st[[1]]});,
      (pllist = ri; stlist = st;)
    ]
  ];
  lplot = ListPlot[pllist,
    PlotMarkers -> {"•", 12},
    PlotStyle -> stlist,
    AxesOrigin -> {0, 0},
    PlotRange -> {{-2. - cmax - 0.2, 2. + cmax + 0.2}, {-ymax, ymax}},
    AspectRatio -> 0.8,
    BaseStyle -> {FontSize -> 14},
    ImageSize -> 72 fsize,
    ImagePadding -> Automatic,
    FrameLabel -> {FontSize -> 14},
    AxesLabel -> {Re[λ], 2 m Im[λ]},
    Epilog -> {
      If[cc > 0,
        Text[ToExpression["c==" <> ToString[cc]], Scaled[{0.85, 0.85}], {-1, 1}],
        Text[ToExpression["c==" <> ToString[0.]], Scaled[{0.85, 0.85}], {-1, 1}]
      ],
      Text[ToExpression["m==" <> ToString[mm]], Scaled[{0.85, 0.95}], {-1, 1}]
    }
  ];
  If[plotest && cc < 2.,
    If[cc > 0,
      Show[lplot, Plot[{Λ[N[cc], Abs[u]], -Λ[N[cc], Abs[u]]},
        {u, -2. + cc, 2. - cc}, PlotStyle -> {{Black}, {Black}}]],
      Show[lplot, Plot[{Λ₀[Abs[u]], -Λ₀[Abs[u]]}, {u, -2., 2.},
        PlotStyle -> {{Black}, {Black}}] ]
    ],
    lplot
  ]
]

(* this function makes a movie for a given m and c changing from cmax to zero
with step -cstep; other parameters are as above *)
MakeFrames[m_, cmax_, cstep_, ymax_, fsize_, plotest_] :=
Module[
  {c},
  ParallelTable[OneFrame[m, c, cmax, ymax, fsize, plotest], {c, cmax, 0., -cstep}]
]

```

```
In[77]:= (* example of a frame *)
OneFrame[100, Sqrt[5] / 2., 2.1, 10, 7.5, True]
```

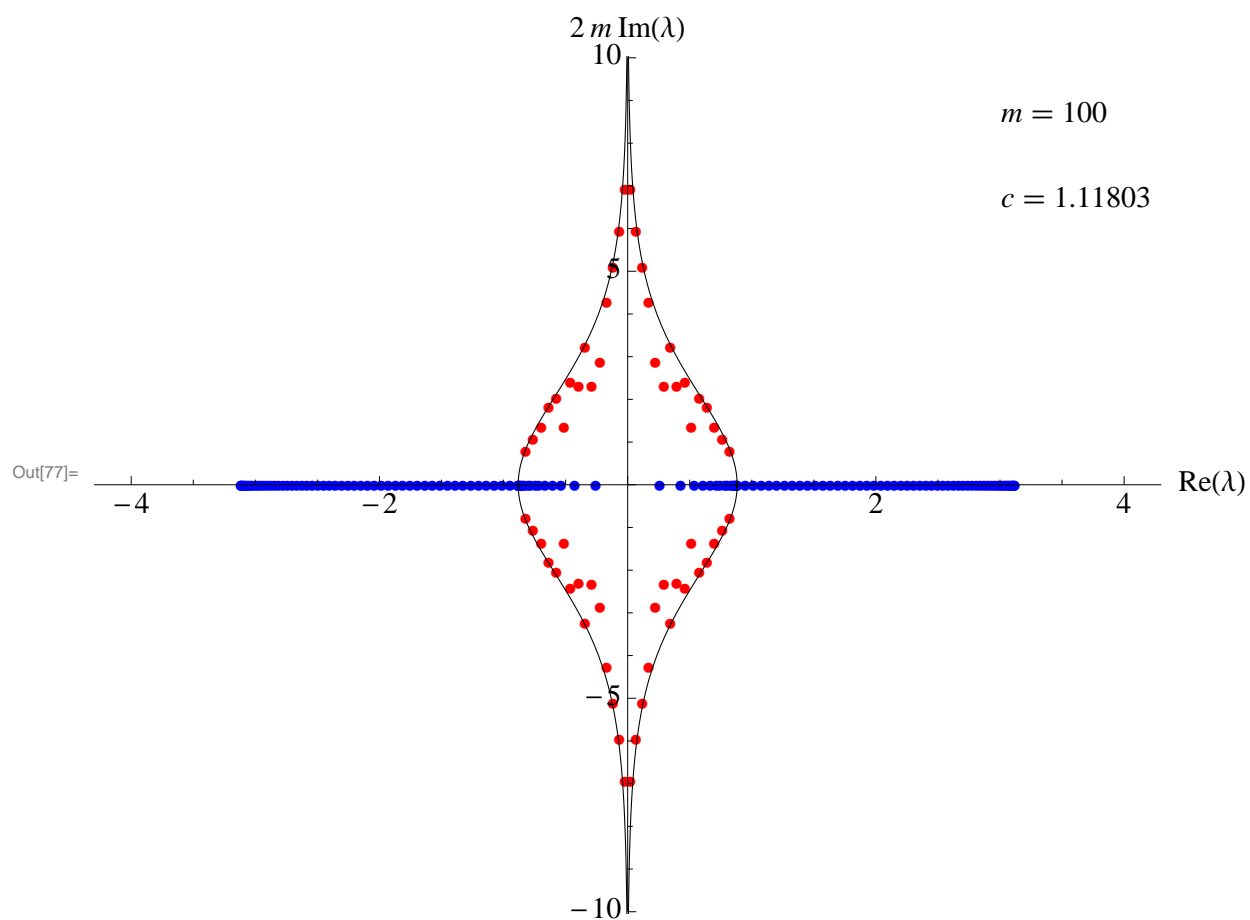

```
(* this operation is slow!*)
frames3 = MakeFrames[100, 2.05, 0.001, 10., 7.5, True] ;

(* Mathematica 7 is unable to export directly to mp4;
conversion from .avi to .mp4 format has been done externally *)

(* this operation is slow!*)
Export["frames3e.avi", frames3, "FrameRate" → 15]
frames3e.avi
```
